# Supplementary material for: Orientation-Disentangled Unsupervised Representation Learning for Computational Pathology
Source: arXiv:2008.11673 source file (2020-08-26)
Supplement: Supplementary file 1 [file appendix.pdf]

# Appendix

## A Class Distributions in TUPAC-ROI

| | Training | Validation | Test |
|---|---|---|---|
| Number of WSIs | 104 | 22 | 22 |
| | | | |
| Tumor Proliferation Grade 1 | 50 (48%) | 11 (50%) | 11 (50%) |
| Tumor Proliferation Grade 2 | 25 (24%) | 5 (23%) | 5 (23%) |
| Tumor Proliferation Grade 3 | 29 (28%) | 6 (27%) | 6 (27%) |
| | | | |
| Pleomorphism Grade 1 | 10 (10%) | 2 (9%) | 3 (13%) |
| Pleomorphism Grade 2 | 43 (41%) | 13 (59%) | 9 (41%) |
| Pleomorphism Grade 3 | 51 (49%) | 7 (32%) | 10 (46%) |

Figure 1: Table summarizing the distributions of each class (tumor proliferation grade and pleomorphism grade) within each split of the TUPAC-ROI dataset.

# B Model Architectures

## B.1 Baseline Variational Auto-Encoder

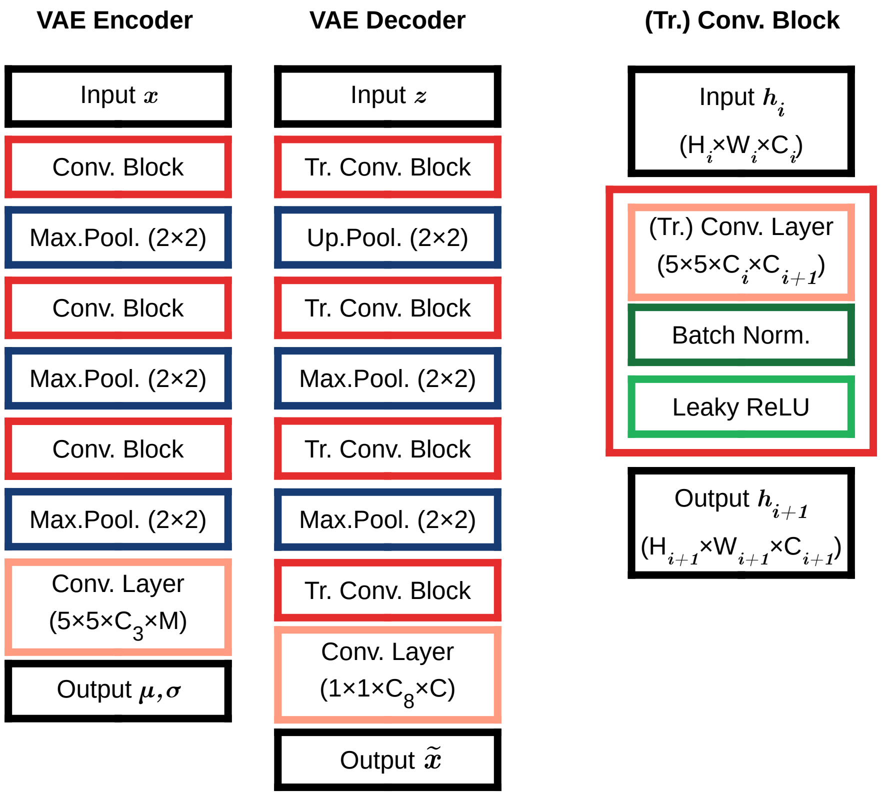


Figure 2: Flowcharts of the encoder and decoder networks implemented to model $q_\phi(\boldsymbol{z}|\boldsymbol{x})$ and $p_\psi(\boldsymbol{x}|\boldsymbol{z})$ in the VAE framework. *Tr.Conv.* indicates *Transposed Convolutions*. We used $C_i = 34$ for $i = 1 \ldots 7$, $C_8 = 32$ and $M = 64$.

## B.2 SE(2,N) Variational Auto-Encoder

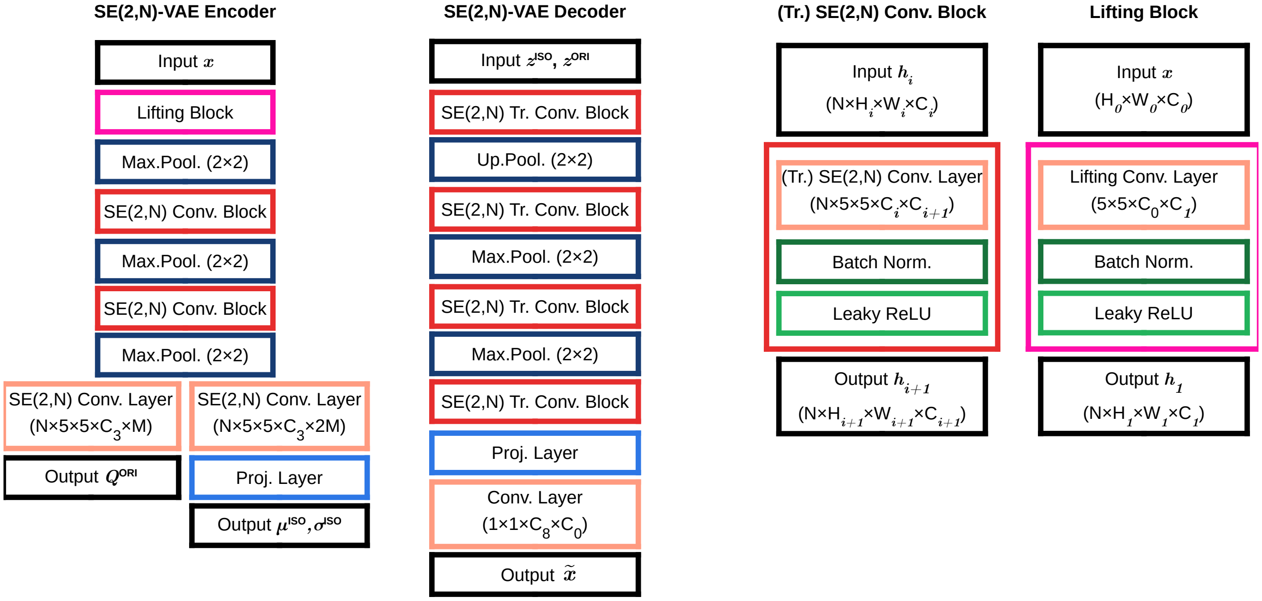


Figure 3: Flowcharts of the proposed encoder and decoder networks implemented to model $q_\phi(\boldsymbol{z}^{ISO}|\boldsymbol{x})$, $q_\phi(\boldsymbol{z}^{ORI}|\boldsymbol{x})$ and $p_\psi(\boldsymbol{x} \mid \boldsymbol{z}^{ISO}, \boldsymbol{z}^{ORI})$. *Tr.Conv.* indicates *Transposed Convolutions*. We used $C_i = 8$ for $i = 1 \ldots 7$, $C_8 = 32$ and $M = 32$.

### B.3 Discriminator

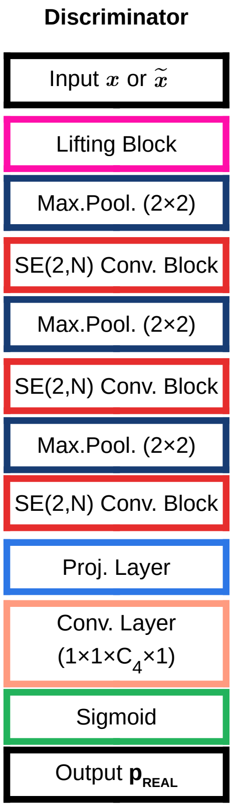


Figure 4: Flowchart of the discriminator network used to extend the reconstruction component of the training objective. We used $C_i = 6$ for $i = 1 \ldots 3$ and $C_4 = 16$.
